# Supplementary material for: Empowering Language Understanding with Counterfactual Reasoning
Source: arXiv:2106.03046 source file (2021-06-06)
Supplement: Supplementary file 1 [file 8_appendix.tex]

\appendix
\section{Reproduction}\label{appsec:hyper_parameter}
In this section, we elaborate the details for reproducing the experiment results.

\subsection{Hyper-parameters of baselines}
We fine-tuned the BERT-based models from the pre-trained Chinese RoBERTa with Whole Word Masking implemented by Huggingface Transformers \cite{Wolf2019HuggingFacesTS} and \cite{cui-2020-revisiting}. For ColBERT, we adopt the original code on Github \footnote{\url{https://github.com/stanford-futuredata/ColBERT}.}. The optimizers for all models are AdamW \cite{loshchilov2017decoupled} implemented by Huggingface Transformers.  
The hyper-parameters for all compared methods are in Table \ref{tab::param_bsln}. 
%``lr'' stands for learning rate. ``bsize'' is batch size. ``accum'' is the gradient accumulation steps. 
``lr'', ``bsize'', ``accum'' stands for learning rate, batch size, and the number of gradient accumulation steps. 
In addition, 
%``scheduler'' represents whether using the linear scheduler of Huggingface Transformers which linearly increases the learning rate from 0 during warmup steps and linearly decreases the learning rate to 0 until trained max steps. 
``scheduler'' indicates the usage of the linear scheduler which linearly increases the learning rate from 0 during warmup steps and linearly decreases the learning rate to 0 until trained max steps. 
% model lr bsize accum scheduler warmup maxsteps 

\begin{table}[h]
\centering
\resizebox{0.48\textwidth}{!}{
\begin{tabular}{lcccccc}
\multicolumn{7}{c}{\cellcolor[HTML]{C0C0C0}Metal} \\
Method & lr & bsize & accum & scheduler & warmup steps & max step \\ \hline \hline
Cla\_M & 1e-5 & 32 & 2 & no & - & - \\
Cla\_S & 1e-4 & 256 & 4 & yes & 150 &  1500 \\ \hline
ColBERT & 1e-4 & 512 & 8 & yes & 100 & 1000 \\
Ret & 1e-4 & 256 & 2 & yes& 150 & 1500 \\
Ret\_QE & 1e-4 & 512 & 8 & yes & 150 & 1500 \\ \hline
\multicolumn{7}{c}{\cellcolor[HTML]{C0C0C0}Agriculture} \\
Method & lr & bsize & accum & scheduler & warmup steps & max step \\ \hline \hline
Cla\_M & 1e-5 & 32 & 2 & no & - & - \\
Cla\_S & 1e-4 & 256 & 2 & yes & 100 & 1000 \\ \hline
ColBERT & 1e-5 & 64 & 2 & yes & 100 & 1000 \\
Ret & 1e-4 & 256 & 2 & yes & 200 & 2000 \\
Ret\_QE & 1e-4 & 128 & 2 & yes & 300 & 3000 \\ \hline
\multicolumn{7}{c}{\cellcolor[HTML]{C0C0C0}Chemical} \\
Method & lr & bsize & accum & scheduler & warmup steps & max step \\ \hline \hline
Cla\_M & 1e-5 & 32 & 2 & no & - & - \\
Cla\_S & 1e-5 & 128 & 2 & yes & 100 & 1000 \\ \hline
ColBERT & 1e-4 & 128 & 4 & yes & 100 & 1000 \\
Ret & 1e-4 & 256 & 2 & yes & 150 & 1500 \\
Ret\_QE & 1e-4& 128 & 2 & yes & 100 & 1000 \\ \hline
\end{tabular}
}    
\caption{Hyper-parameters for document classification and document retrieval methods.}
\label{tab::param_bsln}
\end{table}

%To avoid noise brought from negative news, the training data of Cla\_M is the annotated positive news and the original news from the analyst report, which are labeled by their corresponding queries. 
As can be seen from the table, we did not use scheduler for Cla\_M since Cla\_M is trained very fast and can easily reach good performance. 
It should be noted that the training data of Cla\_M is the annotated positive news and the original news from the analyst report, which are labeled by their corresponding queries. Table \ref{tab::clam_acc} shows the classification accuracy of Cla\_M \wrt the classification on the testing period, which validates the ability of Cla\_M to differentiate news influencing different assets. In addition, due to the consideration of query expansion, Ret\_QE has two additional hyper-parameters where the number of candidate terms for query expansion and the number for expanded terms are set as 30 and 15, respectively. 

% Most of the hyper-parameters are selected based on the best Recall@10 on validation set, since our goal is to provide as much positive news by only looking at the top few news. If Recall@10 has no big difference, we use MAP alternatively. 

% list the training performance of cla m?
% the lambda for hybrid models

\begin{table}[htbp]
\centering
\resizebox{0.3\textwidth}{!}{
\begin{tabular}{lccc}
   & Metal & Agriculture & Chemical \\ \hline \hline
Acc & 0.97 & 0.936 & 0.954\\ \hline
\end{tabular}
}
\caption{Classification accuracy of Cla\_M on the testing set.}
\label{tab::clam_acc}
\end{table}

Furthermore, the proposed hybrid method has an additional hyper-parameter $\lambda$, which adjust the contribution of the classification model. Table \ref{tab::lambda} shows the selected value of $\lambda$ for hybrid models of each dataset.
\begin{table}[htbp]
\centering
\resizebox{0.2\textwidth}{!}{
\begin{tabular}{lcc}
   & Ret\_QE & Ret\\ \hline \hline
Metal & 3 & 0.5 \\
Agriculture & 0.5 & 0.5  \\
Chemical & 0.5& 1 \\ \hline
\end{tabular}
}
\caption{$\lambda$ for hybrid models.}
\label{tab::lambda}
\end{table}

% the hyper-parameters for transfer

Lastly, the All\_Data in the study of transfer learning is trained and validated on the aggregation of three datasets. That is to say, the training (validation) set of the three datasets are aggregated to be the training (validation) set. Upon All\_Data, further fine-tuning on separate datasets becomes All\_Data\_FT. Table~\ref{tab::transfer} shows the hyper-parameters of the fine-tuning procedure for these methods.
%Here we did not apply the scheduler and choose the checkpoint with the best Recall@10 or MAP on validation sets. Table \ref{tab::transfer} lists the settings for transfer study. 

\begin{table}[htbp]
\centering
\resizebox{0.4\textwidth}{!}{
\begin{tabular}{lccc}
   &lr & bsize & accum\\ \hline \hline
ALL\_DATA & 1e-5 & 256 & 4 \\
ALL\_DATA\_FT(Metal) & 1e-5 & 256 & 4  \\
ALL\_DATA\_FT(Agriculture) & 1e-5 & 256 & 4  \\
ALL\_DATA\_FT(Chemical) & 1e-6 & 128 & 2 \\ \hline
\end{tabular}
}
\caption{Hyper-parameters for the study of transfer learning.}
\label{tab::transfer}
\end{table}

It should be noted that the value of hyper-parameters are selected according to the best Recall@10 (\ie Rec10) on validation set, since our goal is to provide as much positive news by only looking at the top few news. It should be noted that, when two combinations tie on Rec10, we select the one with higher MAP.
